# Supplementary material for: Inverting the Kohn-Sham equations with physics-informed machine learning
Source: arXiv:2312.15301 source file (2023-12-23)
Supplement: Supplementary file 1 [file supp.tex]

\begin{figure}[H]
    \centering
    \includegraphics[scale=0.5]{images/both/full set all test one potnetial data driven equi.png}
    \caption{}
    \label{fig:eigerr_complicated}
\end{figure}

\begin{figure}[H]
    \centering
    \includegraphics[scale=0.5]{images/both/full set all test one potnetial PINN equi.png}
    \caption{}
    \label{fig:eigerr_complicated}
\end{figure}

\begin{figure}[H]
    \centering
    \includegraphics[scale=0.5]{images/both/mean error of full dataset PINN vs data driven.png}
    \caption{}
    \label{fig:eigerr_complicated}
\end{figure}

\begin{figure}[H]
    \centering
    \includegraphics[scale=.5]{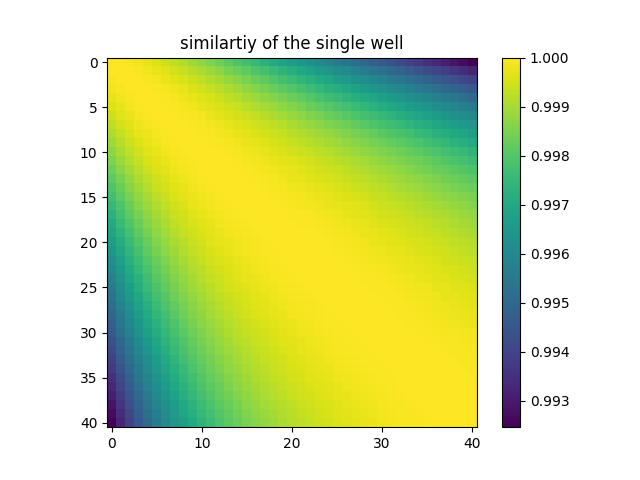}
    \caption{A plot of the cosine similarity of the potentials in the single well data set. The values can range in the range of [0,1].}
    \label{fig:sim_single}
\end{figure}

\begin{figure}[H]
    \centering
    \includegraphics[scale=.5]{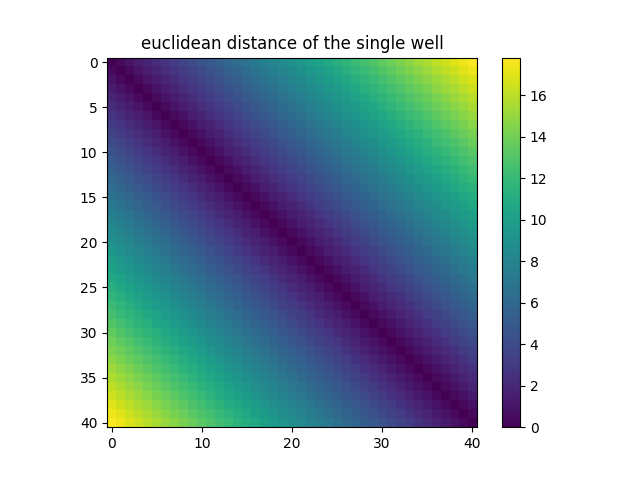}
    \caption{A plot of the euclidean distance of the potentials in the single well data set.}
    \label{fig:sim_single}
\end{figure}

\begin{figure}[H]
    \centering
    \includegraphics[scale=.5]{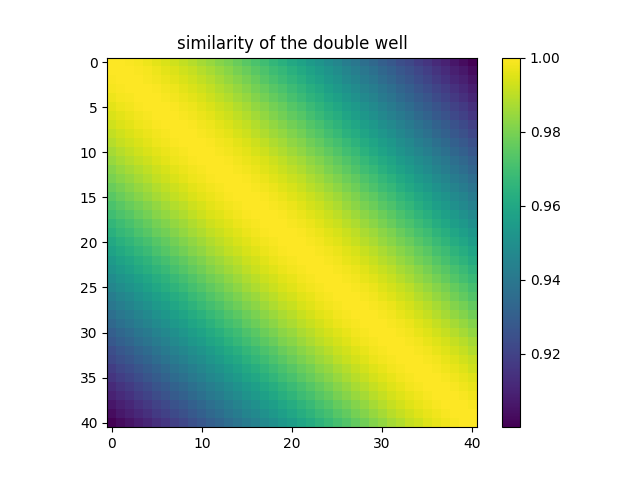}
    \caption{A plot of the cosine similarity of the potentials in the double well data set. The values can range in the range of [0,1].}
    \label{fig:sim_single}
\end{figure}

\begin{figure}[H]
    \centering
    \includegraphics[scale=.5]{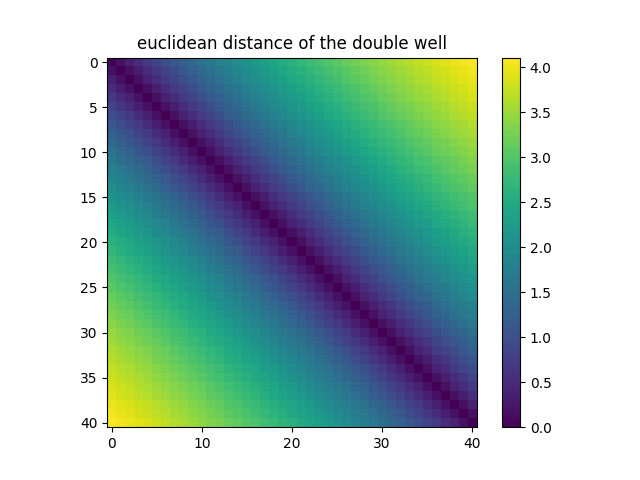}
    \caption{A plot of the euclidean distance of the potentials in the double well data set.}
    \label{fig:sim_single}
\end{figure}

\begin{figure}[H]
    \centering
    \includegraphics[scale=.5]{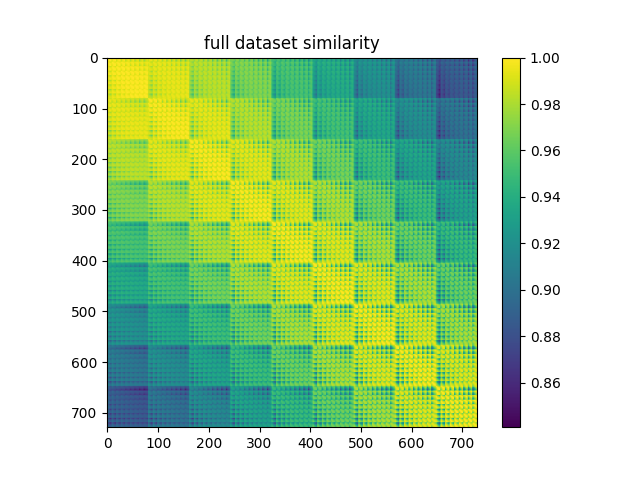}
    \caption{A plot of the cosine similarity of the potentials in the full data set. The values can range in the range of [0,1].}
    \label{fig:sim_single}
\end{figure}

\begin{figure}[H]
    \centering
    \includegraphics[scale=.5]{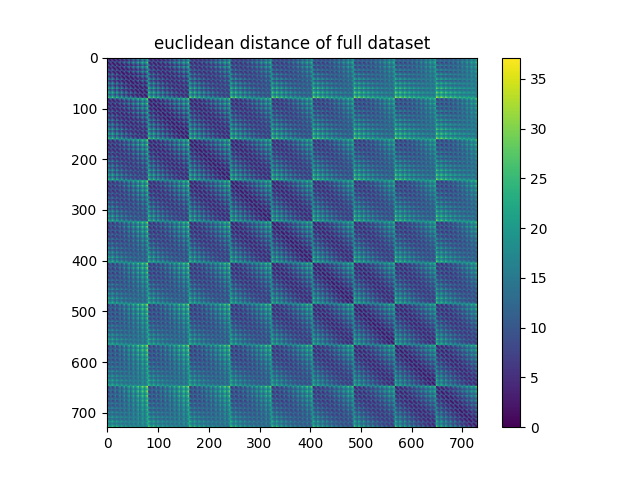}
    \caption{A plot of the euclidean distance of the potentials in the full data set.}
    \label{fig:sim_single}
\end{figure}

\begin{figure}[H]
    \centering
    \includegraphics[scale=.3]{images/depth/Cosinse sim and Euc dist Single well.png}
    \caption{A plot of cosine similarity and euclidean distance of the potentials in the single well data set.}
    \label{fig:sim_single}
\end{figure}

\begin{figure}[H]
    \centering
    \includegraphics[scale=.3]{images/dist/Cosinse sim and Euc dist Double well.png}
    \caption{A plot of cosine similarity and euclidean distance of the potentials in the double well data set.}
    \label{fig:sim_single}
\end{figure}

\begin{figure}[H]
    \centering
    \includegraphics[scale=.3]{images/both/Cosinse sim and Euc dist full.png}
    \caption{A plot of cosine similarity and euclidean distance of the potentials in the fully arying data set.}
    \label{fig:sim_single}
\end{figure}

\begin{figure}[H]
    \centering
    \includegraphics[scale=0.6]{images/depth/varying depth z=2.5.png}
    \caption{A network was randomly initialized 10 times and asked to predict the potential of a 1D well given an input density, The density's first and second derivatives, the depth of the well, and the grid to predict the values on. The input density was 301 points on a grid from -15 to 15. The network had 3 convolutions each with a kernel of 21 and 3 dense layers of 20, 11, and 19 neurons respectively. The residual of the PDE was measured against a vector of zeros use MSE loss. The optimization method was ADAMW. With a learning rate of .0276. the weight for higher energy states were [.0234,.04882]. The network trained on densities resulting from potentials well with a Z value of [2,3,5,6]. The network was stopped early using the density resulting from Z equal to four. The testing Z value shown here is 2.5.}
    \label{fig:z2.5}
\end{figure}

\begin{figure}[H]
    \centering
    \includegraphics[scale=0.6]{images/depth/varying depth z=3.5.png}
    \caption{Shown here is the same network as the previous image. Each initialization is the same as the previous image as well. The only difference is that the network is now predicting the potential that should result in the input density with a charge of Z equal to 3.5.}
    \label{fig:z3.5}
\end{figure}

\begin{figure}[H]
    \centering
    \includegraphics[scale=0.6]{images/depth/variable well depth per error.png}
    \caption{The potentials from the previous two plots were used to calculate their associated set of KS eigenvalues. Each ground truth is also used to calculate a set of eigenvalues. The absolute percent error of the predicted vs ground truth eigenvalues is plotted above for each initialization. The max percent error is about 2.5\% and the min is about .008\%. The mean absolute error for z = 2.5 is .82\% with a standard deviation of .60\%, for z = 3.5 is .75\% with a standard deviation of .58\%, and for all tests in total is .79\% with a standard deviation of .59\%.}
    \label{fig:well_depth_error}
\end{figure}

\begin{figure}[H]
    \centering
    \includegraphics[scale=0.6]{images/depth/variable well depth standard deviation.png}
    \caption{This plot takes the previous one. Uses the mean absolute error to center the data and is made an absolute value plot. Then divides each Z by their respective standard deviation to find the number of standard deviations that each data point is away from the MAE. Removing these data points from the set the MAE error for all data becomes .75\%.}
    \label{fig:well_depth_error}
\end{figure}

\begin{figure}[H]
    \centering
    \includegraphics[scale=0.6]{images/both/well and dist standard deviation.png}
    \caption{The mean absolute error for all data is taken. The standard deviation of all the data points is calculated from the mean. The error plot is centered using the mean and it's absolute value is taken. Then, the data is divided by the standard deviation of 4.52\% to find the number of standard deviations each single prediction is away from the mean. Anything over three standard deviations is marked in red as an outlier. Using the data with the outliers removed the MAE becomes 5.02\%.}
    \label{fig:eigerr_complicated}
\end{figure}

\begin{figure}[H]
    \centering
    \includegraphics[scale=0.6]{images/both/variable z mult per error outlier.png}
    \caption{Here the depth of the well and the distance between the two wells are allowed to vary at the same time. The MAE error for all initializations is 5.29\%. The MAE for each initialization is [4.82, 3.80, 6.90, 6.73, 5.08, 5.83, 3.51, 5.59, 6.39, 4.29]. The network has 6 convolutions, 3 dense layers consisting of 20, 20, and 15 neurons, a kernel of 11, learning rate of .03108, optimizer of ADAMW, and weights for the higher energry states as [.03246, .448989]. This plot is different than the previous ones in that each subplot is now a different initialization where as previously each was a different test case. Here there are 22 cases with different z and d values plotted for each initialization.}
    \label{fig:eigerr_complicated}
\end{figure}

\begin{figure}[H]
    \centering
    \includegraphics[scale=0.6]{images/dist/dist standard deviation.png}
    \caption{A mean absolute error of .72\% and a standard deviation of .66\% were calculated for the absolute percent errors of the network. The absolute percent errors were centered around the mean absolute percent error. Then divided by the standard deviation to calculate the number of standard deviations each data point represents. Any values over three standard deviation are demarcated with red. removing the outliers from the data and recalculating the MAE results in a value of .69\%.}
    \label{fig:my_label}
\end{figure}

\begin{figure}[H]
    \centering
    \includegraphics[scale=0.6]{images/dist/test runs per error.png}
    \caption{A PINN was trained on a small set of data in which the depth of two 1D atomic wells was fixed and the distance between the two wells was varied. The network was then asked to predict the KS potentials for three densities resulting from potentials that the network had not seen before. The potentials that the network predicted were then used to calculate KS eigenfunctions and eigenvalues and and the percent error with the ground truth eigenvalues was predicted. The network was initialized 10 times and the percent error was calculated for the first 6 eigenvalues of the system. The max percent error calculated among the 10 initializations was 2.90\% for a separation of 3.5, for the second eigenvalue, on the 5th initialization.}
    \label{fig:my_label}
\end{figure}

\begin{figure}[H]
    \centering
    \includegraphics[scale=.5]{images/depthxc/MAE of eigenvalues sinle .1 equi no outliers xc.png}
    \caption{The MAE of each eigenvalue after outliers have been removed from the set. The error bars represent three standard deviations from the mean of each eigenvalue.}
    \label{fig:enter-label}
\end{figure}

\begin{figure}[H]
    \centering
    \includegraphics[scale=.5]{images/distxc/MAE of eigenvalues istance .1 xc equi no outliers.png}
    \caption{The MAE of each eigenvalue after outliers have been removed from the set. The error bars represent three standard deviations from the mean of each eigenvalue.}
    \label{fig:enter-label}
\end{figure}

\begin{figure}[H]
    \centering
    \includegraphics[scale=.5]{images/depthxc/difference in error of grid space xc.png}
    \caption{A plot of the mean absolute error of the complete set of predicted potentials on two different grids. Plotted in orange is the the network trained and predicting on a grid of 301 points, and 501 points in blue.}
    \label{fig:grid_error}
\end{figure}

\begin{figure}[H]
    \centering
    \includegraphics[scale=0.35]{images/depthxc/eigenvale absolute and log absolute differnce xc single.png}
    \caption{The charge of a single 1D well is varied between two and six. The data set is in steps of 0.1. 5 points are used for testing and 5 for validation and 31 for training. The absolute difference between predicted and exact eigenvalues is plotted. The ground state error is plotted in blue followed by orange, red, green, purple and brown in increasing energy. the red line is signifies chemical accuracy.}
    \label{fig:well_depth_error}
\end{figure}

\begin{figure}[H]
    \centering
    \includegraphics[scale=0.35]{images/distxc/eigenvale absolute and log absolute differnce xc distance.png}
    \caption{The absolute and logarithm base 10 of the eigenvalue error using potentials predicted by the PINN architecture. The network was trained on a 1D data-set with two soft-coulomb wells of fixed depth. The distance between the wells varied between one and five in steps of 0.1. five points are used for testing, five for validation, and 31 for training. The ground state error is plotted in blue followed by orange, red, green, purple and brown in increasing energy. the red line is signifies chemical accuracy.}
    \label{fig:PINN_dis_error}
\end{figure}

\begin{figure}[H]
    \centering
    \includegraphics[scale=0.35]{images/bothxc/eigenvale absolute and log absolute differnce super super xc full.png}
    \caption{ A single network architecture is trained 10 times to predict KS potentials of a 1D data set. The predicted potentials are used to compute eigenvalues which are compared to exact counterparts. The absolute error and natural log of the absolute error are plotted. The ground state eigenvalue is in blue, then orange, red, green, purple and brown in increasing energy. The red line signifies the limit of chemical accuracy.}
    \label{fig:eigerr_complicated}
\end{figure}

\subsubsection{Varying distance}

Looking to figure \ref{fig:PINN_dis_error} The network performs better when predicting potentials for the data set where the distance between two wells is the only variable. One reason for this is that the systematic error observed in the well depth data set will be small for all distances in this set. This data set exists closer to the left side region of figures \ref{fig:well_depth_error} and \ref{fig:well_depth_error_501}. 
Unlike the single well case though the first excited state's energy is overall greater with a larger spread of returned values. Therefore, the shape of the potential between the bottom and tails of the wells is more varied across predictions. 
The largest error exists at a separation of two but nowhere near a value of .10 as in the single well case with a resolution of 301 points. If the resolution of this set were to increase as before the max error would decrease but probably not at the same rate as  single well 501 point case.
Overall though, the error is less systematic so it is harder to define a single straightforward way to reduce it. The best path forward for improving the error of the double well case is most likely moving to more complex structure of the convolutions used for processing of the density.

\begin{figure}[H]
    \centering
    \includegraphics[scale=0.35]{images/distxc/average eigenvale absolute and log absolute differnce xc distance.png}
    \caption{The second row of \ref{fig:all systems diff PINN} where all of the eigenvalue errors have been averaged.}
    \label{fig:PINN_av_dist_error}
\end{figure}

\begin{table}[H]
  \centering
  \caption{PINN metrics for different experiments (Absolute Error).\\ Chemical accuracy: 1.593e-03 Ha Abs Error}
\begin{tabular}{|l|c|c|}
 \hline
Experiment & Max Abs Error & Mean Abs Error \\
\hline

\hline
dw 301 & 3.36e-3 & 5.15e-4 \\
\hline

\hline
\end{tabular}
\end{table}

\begin{table}[H]
  \centering
  \caption{PINN metrics for different experiments metrics for different experiments (Absolute Percentage Error)}
\begin{tabular}{|l|c|c|}
 \hline
Experiment &  Max Abs \% Error & Mean Abs \% Error \\
\hline

\hline
dw 301 & 4.91e-1 & 1.09e-1 \\
\hline

\hline
\end{tabular}
\end{table}

\begin{figure}[H]
    \centering
    \includegraphics[scale=0.43]{images/two systems diff.png}
    \caption{For the two systems described in the methods section, 10 networks were trained, and the predicted potentials were use to calculate eigenvalues. Errors were plotted as pure absolute difference and on a log base 10 scale. Each eigenvalue level is plotted as its own color. In increasing energy the ordering is blue, orange, red, green, purple, and brown. The energies were calculated in Hartree units.}
    \label{fig:all systems diff PINN}
\end{figure}
